# Supplementary material for: VIBE: Topic-Driven Temporal Adaptation for Twitter Classification
Source: arXiv:2310.10191 source file (2023-11-15)
Supplement: Supplementary file 1 [file appendix.tex]

\section*{Appendix}

% 总述是我们的模型是一个多隐变量的主题模型，多隐变量分别用来表征xys用以去除不相关的噪声因素。为了正确表征xys，我们才用信息瓶颈理论来帮助学习disentangled的表示。我们结合稀疏隐变量和稠密bert特征训练模型引入任务相关信息和时间相关信息，之后用此模型给未来数据打伪标签之后，通过多任务学习将降噪后的过去未来文本表示映射到球空间赋予topic时间意义让模型适应进化中的环境
In this section, we elaborate on the components of our model VIBE shown in figure~\ref{fig:model}. 
We adopt the Neural Topic Model (NTM)~\cite{DBLP:conf/icml/MiaoGB17} to take bag-of-word (bow) vectors of past sentence $o^{x}$ and future sentence $o^{y}$ as input to derive past-exclusive, future-exclusive, and sharing latent topic variables. Two IB regularizers are adopted to force the disentanglement of three latent variables (More explanations in~\ref{ssec:ibr}). 
$z^{s}$ is endowed with task-oriented semantics by inferring the class label $c^{x}$ of past sentence $o^{x}$, meanwhile helps $z^{x}$ and $z^{y}$ capture denoised temporal features. 
% To endow the latent topic variable $z^{s}$ with task-oriented semantics, we concatenate dense feature 
% encoded by BERT~\cite{} and the sparse latent topic feature $z^{s}|o^{x}$ to infer the class label $c^{x}$ of past sentence $o^{x}$. With the fusion training mechanism, 
% The two IB regularizers can capture denoised temporal and task-oriented semantics simultaneously. 
We then employ the trained classifier to pseudo-labeling the future sentence as $c^{y\prime}$. The denoised reconstructed bow of $o^{x}$ and $o^{y}$ feature the time-exclusive topic patterns. We employ multi-task training on inferring timestamps and class labels together to explicitly marry time to topic features in a sphere space. 

\subsection{NTM with Multiple Latent Variables}
A topic model is a statistical model for discovering abstract topics occurring in a collection of texts. Different from the classical framework of NTM with one latent variable, we utilize a new framework of NTM with three latent topic variables to model the joint distribution: samples of paired sentences ($o^{x}$ from the past $X$, $o^{y}$ from the future $Y$) come from the joint distribution ($o^{x}$, $o^{y}$)$\sim$$p_{D}(o^{x},o^{y})$. The three latent topic variables are respectively $z^{x}$ for encoding past-exclusive latent topics, $z^{y}$ for encoding future-exclusive latent topics, and $z^{s}$ for encoding the sharing latent topics between past and future. 
To learn the latent variables, we maximize the marginal likelihood~\cite{diederik2014auto} of the joint distribution of $X$ and $Y$:

\begin{equation}\small
\begin{split}
    p_{\theta}(o^{x},o^{y})=\int dz^{x}dz^{s}dz^{y}p_{\theta_{X}}(o^{x}|z^{x},z^{s})\\
    p_{\theta_{Y}}(o^{y}|z^{y},z^{s})p(z^{x})p(z^{s})p(z^{y})
\end{split}
\end{equation}

The parameter $\theta$=$\left\{ \theta_{X},\theta_{Y} \right\}$ models the conditional distributions. Our training objective is to maximize the generative model $p_{\theta}(o^{x},y^{y})$. Meanwhile, we apply two IB regularizers to force the disentanglement of $Z^{X}$, $Z^{Y}$, and $Z^{S}$. 

\subsection{Task-Oriented Training for NTM}

\subsection{Time-Oriented Training for NTM}

In this section, we elaborate on implementing the information bottleneck regularizers on NTM to learn the time-invariant and -variant latent topic features.
% , which excavates the latent topic features by reconstructing the input bow vector. 
Specifically, the two IB regularizers force the NTM to encode latent topic features exclusively to past and future sentences, and to encode a sharing representation between them.

% The potential of NTM to deal with dynamics comes from its capability of clustering posts exhibiting similar word statistics and forming latent topics to reflect their shared discussion point.
% Therefore, the intra-cluster content, though varying in the generation time,  reflects the implicit semantic consistency throughout time and enables the learning of underlying past-to-future connection.  

\paragraph{Time-Invaraint IB regularizer}
The regularizer disentangles the time-invariant representation $Z^{S}$ and -variant representation $Z^{Y}$/$Z^{Y}$ by the IB regularizer to ensure NTM learns a denoised topic representation sharing by both past and future sentences. $Z^{S}$ is encouraged to be a sharing representation regardless of time information. Interaction information theory (cite) is employed to capture the sharing feature. Interaction information is the generalization of mutual information among three or more random variables, which represents the amount of shared information between them. In our scenario, the interaction information refers to the shared information $Z^{S}$ between past time $X$ and future time $Y$. The formulation for interaction information $I(X;Y;Z^{S})$ go as follows:

\begin{equation}\small
    I(X;Y;Z^{S})=I(X;Z^{S})-I(X;Z^{S}|Y)
\end{equation}
\vspace{-0.5em}
\begin{equation}\small
    I(X;Y;Z^{S})=I(Y;Z^{S})-I(Y;Z^{S}|X)
\end{equation}

In equation~\ref{eq_1}, we maximize the interaction information by maximizing the first term $I(X;Z^{S})$ to make $Z^{S}$ expressive for past time $X$, and minimizing the second term $I(X;Z^{S}|Y)$ to penalize the disturbance from future time $Y$. Symmetrically, equation~\ref{eq_2} encourages $Z^{S}$ to be expressive for future time $Y$ and avoid be affected by past time $X$. By optimizing the two functions simultaneously, $Z^{S}$ is time-invariantly expressive of both $X$ and $Y$. 

\paragraph{Time-Varaint IB regularizer}

We employ regularizers to minimize the mutual information $I(Z^{X};Z^{S})$ and $I(Z^{Y};Z^{S})$, thus time-variant features are statistically independent of the shared features, and vice versa. Here we only present the formulation for past time period $X$, with the analogous future one $Y$.  The mutual information of $Z^{X}$ and $Z^{S}$ go as follows: 

\begin{equation}\small
    I(Z^{X};Z^{S})
    = -I(X;Z^{X},Z^{S})+I(X;Z^{X})+I(X;Z^{S}). 
\end{equation}

mutual information $I(X;Z^{X},Z^{S})$ is maximized to force $Z^{S}$ and $Z^{X}$ to be jointly informative of past time $X$, while penalizes the last two terms to avoid either $Z^{S}$ or $Z^{X}$ to be individually expressive for $X$. 

\paragraph{Joint Regularization for IB Regularizers}
Time-variant and time-invariant representations are jointly regularized. We combine Eq.~\ref{eq_3} and Eq.~\ref{eq_5} for time X regularization, as time Y is analogous. 

\begin{equation}\small
\begin{array}{rl}
\max\limits_q & I\left(X ; Y ; Z^S\right)-I\left(Z^X ; Z^S\right) \\
& =\underbrace{\cancel{I\left(X, Z^S\right)}-I\left(X ; Z^S \mid Y\right)}_{I\left(X ; Y ; Z^S\right)}\\
&+\underbrace{I\left(X ; Z^X, Z^S\right)-I\left(X ; Z^X\right)-\cancel{I\left(X, Z^S\right)}}_{-I\left(Z^X ; Z^S\right)} \\
& =I\left(X ; Z^X, Z^S\right)-I\left(X ; Z^X\right)-I\left(X ; Z^S \mid Y\right) .
\end{array}
\end{equation}

\vspace{-0.5em}
\begin{equation}\small
\begin{array}{rl}
\max\limits_q & I\left(X ; Y ; Z^S\right)-I\left(Z^Y ; Z^S\right) \\
& =I\left(Y ; Z^Y, Z^S\right)-I\left(Y ; Z^Y\right)-I\left(Y ; Z^S \mid Y\right) .
\end{array}
\end{equation}

\paragraph{Tractable Optimization for IB Regularizers}
Since there are intractable integrals like unknown distribution $p_{D}(o^{x},o^{y})$ in mutual information terms mentioned before, we maximize generative distributions' lower bounds for tractability. 

For $I(X;Z^{X};Z^{Y})$, we derives its lower bound with the generative distribution $p(o^{x}|z^{x},z^{s})$ as follows:

\begin{equation}\small
\begin{aligned}
I\left(X ; Z^X,Z^S\right)=\mathbb{E}_{q\left(z^x, z^s \mid x\right) p_D(x)}\left[\log \frac{q\left(x \mid z^x, z^s\right)}{p_D(x)}\right] \\
=H(X)+\mathbb{E}_{q\left(z^x, z^s \mid x\right) p_D(x)}\left[\log p\left(x \mid z^x, z^s\right)\right]\\
+\mathbb{E}_{q\left(z^x, z^s\right)}\left[D_{K L}\left[q\left(x \mid z^x, z^s\right) \| p\left(x \mid z^x, z^s\right)\right]\right] \\
\geq H(X)+\mathbb{E}_{q\left(z^x, z^s \mid x\right) p_D(x)}\left[\log p\left(x \mid z^x, z^s\right)\right] \\
=H(X)+\mathbb{E}_{p_D(x, y) q\left(z^x \mid x\right) q\left(z^s \mid x, y\right)}\left[\log p\left(x \mid z^x, z^s\right)\right]
\end{aligned}
\end{equation}

Additional to the maximization of $I(X;Z^{X};Z^{Y})$, Eq.~\ref{eq_8} fits $p(o^{x}|z^{x},z^{s})$ to $q(o^{x}|z^{x},z^{s})$ so that we can use it as a decoder. 

For intractable $-I(X;Z^{X})$ (unknow distribution $p_{D}(o^{x})$), the generative distribution $p(z^{x})$ is adopted as the standard Gaussian, known as the Variational Information Bottleneck (VIB) (cite). The lower bound go as follows:

\begin{equation}\small
    -I(X;Z^{X})\geq -\mathbb{E}_{PD(x)}\left[D_{K L}\left[q\left(z^x\mid x \right) \| p\left(z^s\right)\right]\right]
\end{equation}

Similar to VIB, the lower bound for $-I(X;Z^{S}|Y)$ go as follows:

\begin{equation}\small
\begin{aligned}
-I\left(X ; Z^S \mid Y\right) & =-\mathbb{E}_{p_D(x, y) q\left(z^s \mid x, y\right)}\left[\log \frac{q\left(z^s \mid x, y\right)}{q\left(z^s \mid y\right)}\right] \\
% & =-\mathbb{E}_{p_D(x, y) q\left(z^s \mid x, y\right)}\left[\log \frac{q\left(z^s \mid x, y\right) r^y\left(z^s \mid y\right)}{r^y\left(z^s \mid y\right) q\left(z^s \mid y\right)}\right] \\
% & =-\mathbb{E}_{p_D(x, y)}\left[D_{K L}\left[q\left(z^s \mid x, y\right) \| r^y\left(z^s \mid y\right)\right]\right]+\mathbb{E}_{p_D(y)}\left[D_{K L}\left[q\left(z^s \mid y\right) \| r^y\left(z^s \mid y\right)\right]\right] \\
& \geq-\mathbb{E}_{p_D(x, y)}\left[D_{K L}\left[q\left(z^s \mid x, y\right) \| r^y\left(z^s \mid y\right)\right]\right]
\end{aligned}
\end{equation}

Substituting Eq.~\ref{eq_8}-\ref{eq_10} to Eq.\ref{eq_6}-\ref{eq_7}, we get the lower bound as follows:

\begin{equation}\small
\begin{aligned}
&(\left.\left(X ; Y ; Z^S\right)-I\left(Z^X ; Z^S\right)\right)+\left(I\left(X ; Y ; Z^S\right)-I\left(Z^Y ; Z^S\right)\right) \\
% &= 2 \cdot I\left(X ; Y ; Z^S\right)-I\left(Z^X ; Z^S\right)-I\left(Z^Y ; Z^S\right) \\
&= I\left(X ; Z^X, Z^S\right)+I\left(Y ; Z^Y, Z^S\right)-I\left(X ; Z^X\right)-I\left(Y ; Z^Y\right)-I\left(X ; Z^S \mid Y\right)-I\left(Y ; Z^S \mid X\right) \\
& \geq \mathbb{E}_{p_D(x, y)}\left[\mathbb{E}_{q\left(z^s \mid x, y\right) q\left(z^x \mid x\right)}\left[\log p\left(x \mid z^x, z^s\right)\right]+\mathbb{E}_{q\left(z^s \mid x, y\right) q\left(z^y \mid y\right)}\left[\log p\left(y \mid z^y, z^s\right)\right]\right] \\
&-\mathbb{E}_{p_D(x, y)}\left[D_{K L}\left[q\left(z^x \mid x\right) \| p\left(z^x\right)\right]+D_{K L}\left[q\left(z^y \mid y\right) \| p\left(z^y\right)\right]\right] \\
& \quad-\mathbb{E}_{p_D(x, y)}\left[D_{K L}\left[q\left(z^s \mid x, y\right) \| r^y\left(z^s \mid y\right)\right]+D_{K L}\left[q\left(z^s \mid x, y\right) \| r^x\left(z^s \mid x\right)\right]\right] \\
& \quad+H(X)+H(Y)
\end{aligned}
\end{equation}

To integrate the joint regularization on the disentanglement of past time $X$ and future time $Y$, and the maximum likelihood objective in Eq. (cite), we combine them as a joint maximization objective as follows:

\begin{equation}\small
\begin{aligned}
& \max _{p, q} \mathbb{E}_{q\left(z^x, z^s, z^y, x, y\right)}\left[\log \frac{p\left(x, y, z^x, z^s, z^y\right)}{q\left(z^x, z^s, z^y \mid x, y\right)}\right]\\
&+\lambda\left(2 \cdot I\left(X ; Y ; Z^S\right)-I\left(Z^X ; Z^S\right)-I\left(Z^Y ; Z^S\right)\right) \\
& \geq \max _{p, q, r}(1+\lambda) \cdot \mathbb{E}_{p_D(x, y)}[E L B O(p, q)] \\
& \quad+\lambda \cdot \mathbb{E}_{p_D(x, y)}\left[D_{K L}\left[q\left(z^s \mid x, y\right) \| p\left(z^s\right)\right]\right] \\
& \quad-\lambda \cdot \mathbb{E}_{p_D(x, y)}\left[D_{K L}\left[q\left(z^s \mid x, y\right) \| r^y\left(z^s \mid y\right)\right]+D_{K L}\left[q\left(z^s \mid x, y\right) \| r^x\left(z^s \mid x\right)\right]\right]
\end{aligned}
\end{equation}

\subsection{Joint Training for NTM}

\subsection{Topic Sphere Space Mapping}
Since $o_x$ and $o_y$' reconstructed bow vectors are based on a ruthless vocabulary dictionary, sentences with similar semantics are not close in feature space. To tackle this issue, we map the denoised reconstructed bow vectors of $o_x$ and $o_y$ into a sphere space by multi-task training on predicting timestamps and class labels of $o_x$ and $o_y$ at the same time.
